# Supplementary material for: A Class of Multirate Infinitesimal GARK Methods
Source: arXiv:1808.02759 source file (2022-02-01)
Supplement: Supplementary file 2 [file appendix_useful_formulas.tex]

\section{Useful formulas}
\begin{equation*}
\begin{split}
(\A^{\{\f,\f\}} \c^{\{\f\}})_{i} &=
\sum_{j=1}^{i-1}  c_{j}^{\{\s\}} \Delta c^{\{\s\}}_{j} \, \one^{\{\f\}}  b^{\{\f\}}\,^T  \, \one^{\{\f\}} \\
&+ \sum_{j=1}^{i-1}   \bigl( \Delta c^{\{\s\}}_{j} \bigr)\,^2\, \one^{\{\f\}}  b^{\{\f\}}\,^T
\,\c^{\{\f\}} \\
&+c_{i}^{\{\s\}}  \, \Delta c_{i}^{\{\s\}}\, A^{\{\f\}} \, \one^{\{\f\}} \\
&+ \left(\Delta c_{i}^{\{\s\}}\right)^2\, A^{\{\f\}}\,\c^{\{\f\}} \\
&=
\frac{1}{2} c_{i}^{\{\s\}}\,^2\, \one^{\{\f\}} +c_{i}^{\{\s\}}  \, \Delta c_{i}^{\{\s\}}\, c^{\{\f\}}  + \bigl(\Delta c_{i}^{\{\s\}}\bigr)^2\, A^{\{\f\}}\,c^{\{\f\}} 
\end{split}
\end{equation*}
\begin{eqnarray*}
\A^{\{\f,\s,i\}}\, \c^{\{\s\}} &=& \begin{blockarray}{ccccc}
\scriptstyle 1 \le j  \le i-1 & \scriptstyle       i &  \scriptstyle       i+1 & &\scriptstyle  s^{\{\s\}} \\
\begin{block}{[ccccc]}
a_{i,j}^{\{\s\}}\,\one^{\{\f\}} \, 
+ \sum_{k \ge 0} \gamma_{i,j}^k (A^{\{\f\}} \, c^{\{\f\}}\,^{\times k}) &  \sum_{k \ge 0} \gamma_{i,i}^k (A^{\{\f\}} \, c^{\{\f\}}\,^{\times k}) &\scriptstyle  0 & \cdots  &  0 \\ 
\end{block}\end{blockarray} \\
&=& \sum_{j=1}^{i-1} a_{i,j}^{\{\s\}}\,c_{j}^{\{\s\}}\,\one^{\{\f\}}
+ \sum_{k \ge 0} \sum_{j=1}^{i} c_{j}^{\{\s\}}\,\gamma_{i,j}^k\, (A^{\{\f\}} \, c^{\{\f\}}\,^{\times k}) \\
&=& \one^{\{\f\}}\, \big(A^{\{\s\}}\,c^{\{\s\}}\big)_{i,:} + \sum_{k \ge 0} \big(A^{\{\f\}} \, c^{\{\f\}}\,^{\times k}\big)\, \big(\boldsymbol{\Gamma}^k\, c^{\{\s\}}\big)_{i,:}
\end{eqnarray*}

Second $C(1,1)$ condition:
\begin{equation*}
\begin{split}
\A^{\{\s,\f\}} \c^{\{\f\}} &=
\sum_{i=1}^{s^{\{\s\}}}  
\left(c_{i+1}^{\{\s\}}-c_{i}^{\{\s\}}\right)\, \mathbf{g}_{i+1} b^{\{\f\}}\,^T \,\left( c_{i}^{\{\s\}}  \, \one^{\{\f\}} +  \Delta c^{\{\s\}}_{i} \,c^{\{\f\}} \right) \\
&=
\frac{1}{2}\,\sum_{i=1}^{s^{\{\s\}}}  
\left(c_{i+1}^{\{\s\}}c_{i}^{\{\s\}}-c_{i}^{\{\s\}}\,^2 + \frac{c^{\{\s\}}_{i+1}\,^2-2c^{\{\s\}}_{i+1}c^{\{\s\}}_{i} + c^{\{\s\}}_{i}\,^2}{2}\right)\, \mathbf{g}_{i+1}  \\
&=
\frac{1}{2}\,\c^{\{\s\}}\,^{\times 2} \\
&= \A^{\{\s,\s\}} \c^{\{\s\}}
\end{split}
\end{equation*}
It cannot be satisfied by an explicit slow method.
\end{theorem}

\begin{theorem}[D(1,1) simplifying conditions]
First $D(1,1)$ condition:
\begin{equation*}
\begin{split}
(\b^{\{\f\}}\,^T\,\A^{\{\f,\f\}} )_{i} &=\bigl( \Delta c^{\{\s\}}_{j} \bigr)^2\,b^{\{\f\}}\,^T\,A^{\{\f\}}
+ \sum_{j=i+1}^{s^{\{\s\}}}  \bigl( \Delta c^{\{\s\}}_{j}\bigr)^2\,b^{\{\f\}}\,^T \\
&=\big( \Delta c_{i}^{\{\s\}} \big)^2\,b^{\{\f\}}\,^T\,A^{\{\f\}}
+ \sum_{j=i+1}^{s^{\{\s\}}} \big( \Delta c_{j}^{\{\s\}}\big)^2\,b^{\{\f\}}\,^T
\end{split}
\end{equation*}
\begin{equation*}
\begin{split}
\b^{\{\s\}}\,^T\,\A^{\{\s,\f,i\}} &= \left(c_{i+1}^{\{\s\}}-c_{i}^{\{\s\}}\right)\, b^{\{\s\}}\,^T\,\mathbf{g}_{i+1} b^{\{\f\}}\,^T \\
&= \left(c_{i+1}^{\{\s\}}-c_{i}^{\{\s\}}\right)\, \left( \sum_{\ell=i+1}^{s^{\{\s\}}} b_\ell^{\{\s\}}\right) b^{\{\f\}}\,^T
\end{split}
\end{equation*}
Second $D(1,1)$ condition:
Let
\begin{equation*}
\zeta_k \coloneqq b^{\{\f\}}\,^T\,A^{\{\f\}} \, c^{\{\f\}}\,^{\times k}.
\end{equation*}
\begin{equation*}
\begin{split}
\b^{\{\f\}}\,^T\,\A^{\{\f,\s\}} &= 
\sum_{i=1}^{s^{\{\s\}}}  \left(c_{i+1}^{\{\s\}}-c_{i}^{\{\s\}}\right)  
\begin{blockarray}{ccccc}
\scriptstyle 1 \le j  \le i-1 & \scriptstyle       i &  \scriptstyle       i+1 & &\scriptstyle  s^{\{\s\}} \\
\begin{block}{[ccccc]}
a_{i,j}^{\{\s\}} \, 
+ \sum_{k \ge 0} \gamma_{i,j}^k \,\zeta_k &  \sum_{k \ge 0} \gamma_{i,i}^k \, \zeta_k &\scriptstyle  0 & \cdots  &  0 \\ 
\end{block}\end{blockarray} \\
\b^{\{\s\}}\,^T\,\A^{\{\s,\s\}} &= \sum_{i=j+1}^{s^{\{\s\}}} b^{\{\s\}}_i\, a^{\{\s\}}_{i,j}
\end{split}
\end{equation*}
\begin{equation*}
\begin{split}
\b^{\{\f\}}\,^T\,\A^{\{\f,\s\}} &= 
\Delta c^{\{\s\}}\,^T \, \left( A^{\{\s\}} +   \sum_{k \ge 0} \zeta_k\,\boldsymbol{\Gamma}^k \right)
\end{split}
\end{equation*}

\end{theorem}
